# Supplementary material for: Interacting models for twisted bilayer graphene: a quantum chemistry approach
Source: arXiv:2211.09243 source file (2022-11-16)
Supplement: Supplementary file 1 [file appendix2.tex]

\section{Treatment of antiunitary symmetry operations}
\label{sec:antiunitary}
We now consider the case of anti-unitary symmetries. Recall that any anti-unitary symmetry may be written as $\wt{g} = g \mc{K}$ and hence the primitive creation operators transform as:
\begin{equation}
\begin{split}
    (g \mc{K} \hat{c}_{\vk}^\dag (g \mc{K})^{-1})(\alpha) & = \sum_{\alpha'} \hat{c}_{g\vk}^\dag(\alpha') [D(g)]_{\alpha',\alpha} \\
    (g \mc{K} \hat{c}_{\vk} (g \mc{K})^{-1})(\alpha) & = \sum_{\alpha'} \hat{c}_{g\vk}(\alpha') [D(g)]_{\alpha',\alpha}^{*}
\end{split}
\end{equation}
Now we can calculate the action of this operation on any quadratic Hamiltonian in the primitive basis $\hat{H}=\sum_{\vk}\sum_{\alpha,\beta}[h(\vk)]_{\alpha\beta} \hat{c}^{\dag}_{\vk}(\alpha) \hat{c}_{\vk}(\beta)$. In particular
\begin{equation}
\begin{split}
(g \mc{K}) \hat{H} (g \mc{K})^{-1}=&g \mc{K} \sum_{\vk} \sum_{\alpha\beta}[h(\vk)]_{\alpha\beta} \hat{c}^{\dag}_{\vk}(\alpha) \hat{c}_{\vk}(\beta)\mc{K} g^{-1}\\
=& \sum_{\vk} \sum_{\alpha\beta} \sum_{\alpha'\beta'}[h^*(\vk)]_{\alpha\beta} \hat{c}^{\dag}_{g\vk}(\alpha') [D(g)]_{\alpha',\alpha} \hat{c}_{g\vk}(\beta') [D(g)]^*_{\beta',\beta}\\
=& \sum_{\vk} [D(g)h^*(\vk)D^{\dag}(g)]_{\alpha'\beta'}\hat{c}^{\dag}_{g\vk}(\alpha') \hat{c}_{g\vk}(\beta').
\end{split}
\end{equation}

If $\hat{H}$ is invariant under $\wt{g}$, i.e., $\wt{g}\hat{H}\wt{g}^{-1}=\hat{H}$, then this calculation shows that at the matrix level:
\begin{equation}
D(g) h^*(\vk)=h(g\vk) D(g).
\end{equation}
In other words, 
\begin{equation}
h(g\vk)D(g)u^*_{n\vk}=D(g)h^*(\vk)u^*_{n\vk}=\varepsilon_{n\vk} D(g)u^*_{n\vk},
\end{equation}
or equivalently $D(g)u^*_{n\vk}$ is an eigenfunction of $h(g\vk)$ with the eigenvalue $\varepsilon_{n,g\vk}=\varepsilon_{n\vk}$. Hence, similar to the unitary case, we can define a ``sewing matrix'', $[B(g)]_{\vk}$,
\begin{equation}
%\label{eqn:matrix_representation} Doubly defined but not referred! 
(D(g) u^*_{n\vk})(\alpha)=
\sum_{\alpha'} [D(g)]_{\alpha,\alpha'} u^*_{n\vk}(\alpha')=
\sum_{m}  u_{m,g\vk}(\alpha) [B(g)]_{\vk,mn}.
\end{equation}
Here
\begin{equation}
[B(g)]_{\vk,mn}=\braket{u_{m,g\vk} | D(g) | u^*_{n\vk}},
\end{equation}
where the bra-ket notation denotes contraction over the internal indices $\alpha,\alpha'$.
Similar to the unitary case, when the system is gapped, it is easily verified that $[B(g)]_{\vk}$ is a unitary matrix using a contour integral argument (see Appendix \ref{sec:contour-argument}). Given the definition of sewing matrices, one can calculate that:
\begin{equation}
\begin{split}
g \mc{K} \hat{f}^{\dag}_{n\vk} \mc{K} g^{-1}=&\sum_{\alpha}  g\hat{c}_{\vk}^{\dagger}(\alpha) g^{-1}u^*_{n\vk}(\alpha')\\
=&\sum_{\alpha,\alpha'}  \hat{c}^{\dag}_{g\vk}(\alpha')[D(g)]_{\alpha',\alpha}
u^*_{n\vk}(\alpha)\\
=& \sum_{\alpha'} \hat{c}^{\dag}_{g\vk}(\alpha') \sum_{m} u_{m,g\vk}(\alpha') [B(g)]_{\vk,mn} \\
=& \sum_{m} \hat{f}^{\dag}_{m,g\vk}  [B(g)]_{\vk,mn},
\end{split}
\label{eqn:sewing_transf_antiunitary}
\end{equation}
which is of the same form as the unitary case in~\cref{eqn:sewing_transf_unitary}.

We now turn to verify the analog of \cref{eqn:order-parameter} for anti-unitary symmetries %\LL{ should we be consistent with the convention of complex conjugation, i.e., $\overline{a}$ vs $a^*$?} \kds{True, I don't usually use ${}^*$ for complex conjugation so I forgot}
\begin{equation}
\begin{split}
[P(\vk)]_{nm}=&\braket{\Psi|\hat{f}^{\dag}_{m\vk} \hat{f}_{n\vk}|\Psi}=\Tr[\hat{f}^{\dag}_{m\vk} \hat{f}_{n\vk}\ket{\Psi}\bra{\Psi}]\\
=&\Tr[\hat{f}^{\dag}_{m\vk} \hat{f}_{n\vk}\mc{K} g^{-1}g \mc{K} \ket{\Psi}\bra{\Psi}\mc{K}g^{-1} g \mc{K}]\\
=&\braket{\Psi|g\mc{K}\hat{f}^{\dag}_{m\vk} \hat{f}_{n\vk}\mc{K} g^{-1}|\Psi}^*\\
=&\sum_{pq} [B(g)]^*_{\vk,pm} [B(g)]_{\vk,qn} \braket{\hat{f}^{\dag}_{p,g\vk} \hat{f}_{q,g\vk}}^*=([B(g)]_{\vk}^{\top}P(g\vk)^*[B(g)]_{\vk}^*)_{nm}.
\end{split}
\end{equation}
Therefore, the corresponding order parameter for antiunitary symmetries is
\begin{equation}
\begin{split}
\mc{C}_{\vk}(\wt{g}) = \mc{C}_{\vk}(g \mc{K})
& = \|  [B(g)]_{\vk}^{\top}P(g\vk)^*[B(g)]_{\vk}^* - P(\vk) \| \\
& = \|  P(g\vk)[B(g)]_{\vk} - [B(g)]_{\vk} P(\vk)^* \| 
\end{split}
\end{equation}
where in the last line we have used that complex conjugation preserves unitarily invariant norms.

To see that this quantity is gauge invariant, first recall that from the main text (Eq. \eqref{eq:1rdm-gauge}) we showed that under a gauge transformation the 1-RDM transforms as 
\begin{equation}
    [P(\vk)]_{nm} \mapsto [U(\vk)^\dagger P(\vk) U(\vk)]_{nm}
\end{equation}
Hence, to show gauge invariance we only need to calculate how the sewing matrices transform in this case. By definition under a gauge transformation we have
\begin{equation}
\begin{split}
[B(g)]_{\vk,mn} & \mapsto \sum_{m'n'} [U(g\vk)]_{mm'}^* [U(g\vk)]_{m'm} [U(g\vk)]_{nn'} \braket{u_{m',g\vk} | D(g) | u^*_{n\vk}} \\
& =  (U(g\vk)^{\dagger}B(g)_{\vk}U(\vk)^*)_{mn}
\end{split}
\end{equation}

%one can easily check \LL{ as a general rule of thumb, I would like to always avoid a sentence like "one can easily / it is easy to..."} \kds{Ok. I was a little tired when I was writing this section. Fixing this now.} that under a gauge transformation
Hence
\begin{equation}
\begin{split}
    P(g\vk) [B(g)]_{\vk} \mapsto & U(g\vk)^\dagger P(g\vk) U(g\vk) U(g\vk)^{\dagger} [B(g)]_{\vk} U(\vk)^* \\
    [B(g)]_{\vk} P(\vk)^* \mapsto & U(g\vk)^\dagger  [B(g)]_{\vk} U(\vk)^* U(\vk)^\top P(\vk)^* U(\vk)^*
\end{split}
\end{equation}
which implies that
\begin{equation}
\begin{split}
\mc{C}_{\vk}(\wt{g}) & \mapsto \| U(g\vk)^\dagger P(g\vk) [B(g)]_{\vk} U(\vk)^* - U(g\vk)^\dagger  [B(g)]_{\vk} P(\vk)^* U(\vk)^* \| \\
& = \| P(g\vk) [B(g)]_{\vk} -  [B(g)]_{\vk} P(\vk)^* \|.
\end{split}
\end{equation}
This proves that $\mc{C}_{\vk}(\wt{g})$ is gauge invariant.

\section{Unitarity of the sewing matrix}
\label{sec:contour-argument}
Suppose that we are given a single body Hamiltonian $h(\vk)$ with corresponding eigenvectors/eigenvalue pairs $\{ (u_{n\vk}(\alpha), \epsilon_{n\vk}) \}$ where $\vk \in BZ$ and $\alpha$ is a multi-index running over the additional degrees of freedom (in this work, sublattice, layer, valley, spin). Suppose further that there exists a set of occupied orbitals, $\mc{I}_{occ}$, whose energies are separated from the rest by an energy gap. That is, there exists a constant $c$ such that for all $\vk$ we have the gap condition
\[
\min_{n \in \mc{I}_{occ}} \min_{m \not\in \mc{I}_{occ}} | \epsilon_{n\vk} - \epsilon_{m\vk} | \geq c > 0.
\]
\kds{This assumption is a bit more restrictive but it makes the proof easier.} Under this assumption, we will prove that the sewing matrix $[B(g)]_{\vk}$ defined in Eq. \eqref{sec:sewing-def} is unitary.

We first consider case where $g$ is a unitary symmetry. In this case, it suffices to show that the set $\{ D(g) \ket{u_{n\vk}} : n \in \mc{I}_{occ} \}$ and the set $\{ \ket{u_{n,g\vk}} : n \in \mc{I}_{occ} \}$ are two different orthonormal bases for the same space. Due to our gap assumption, the occupied projector $P_{occ}$ can be written a sum of exterior products:
\[
P_{occ}(\vk) = \sum_{n \in \mc{I}_{occ}} | u_{n\vk} \rangle \langle u_{n\vk} |.
\]
By the Riesz projection formula, we can also represent the occupied projector as a contour integral
\[
P_{occ}(\vk) = \frac{1}{2 \pi i} \int_{\mc{C}} (z - h(\vk))^{-1} dz
\]
where $\mc{C}$ is a closed contour in the complex plane enclosing the eigenvalues $\{ \epsilon_{n\vk} : n \in \mc{I}_{occ} \}$. Conjugating both sides by the representation matrix $D(g)$ then gives that
\begin{equation}
\begin{split}
    D(g) P_{occ}(\vk) (D(g))^\dagger & = \frac{1}{2 \pi i} \int_{\mc{C}} D(g) (z - h(\vk))^{-1} (D(g))^\dagger dz \\
    & = \frac{1}{2 \pi i} \int_{\mc{C}} \Big((z - D(g) h(\vk) (D(g))^\dagger\Big)^{-1} dz \\
    & = \frac{1}{2 \pi i} \int_{\mc{C}} (z - h(g\vk) )^{-1} dz \\
    & = P_{occ}(g\vk).
\end{split}
\end{equation}
Hence
\[
P_{occ}(g\vk) =  \sum_{n \in \mc{I}_{occ}} D(g) | u_{n\vk} \rangle \langle u_{n\vk} | (D(g))^\dagger.
\]
Since $D(g)$ is unitary, it follows that $P_{occ}(\vk)$ and $P_{occ}(g\vk)$ have the same rank and $\{ D(g) \ket{u_{n\vk}} : n \in \mc{I}_{occ} \}$ is a complete orthogonal basis for the range of $P_{occ}(g\vk)$, completing the argument

If instead $g$ is antiunitary, there exists an analog of the sewing matrix \LL{ should we just call it a sewing matrix instead of an analogue?} \kds{Sure.} (see Appendix \ref{sec:antiunitary}) which we can also show is unitary. In this case, we instead consider $P_{occ}(\vk)^*$ which is also given by taking the complex conjugation of the Riesz projection formula:
\begin{equation}
P_{occ}(\vk)^* = \frac{-1}{2 \pi i} \int_{\mc{C}} (\overline{z} - h^{*}(\vk))^{-1} dz
\end{equation}
We may assume without loss of generality that the contour $\mc{C}$ is symmetric about the real axis, therefore performing the change of variables $z \mapsto \overline{z}$ and reversing the orientation of the contour we conclude that
\begin{equation}
P_{occ}(\vk)^* = \frac{1}{2 \pi i} \int_{\mc{C}} (z - h^{*}(\vk))^{-1} dz.
\end{equation}
Finally, conjugating by $D(g)$ gives us that
\begin{equation}
\begin{split}
    D(g) P_{occ}(\vk)^* (D(g))^\dagger
    & = \frac{1}{2 \pi i} \int_{\mc{C}} (z - D(g) h^*(\vk)(D(g))^\dagger)^{-1}  dz \\
     & = \frac{1}{2 \pi i} \int_{\mc{C}} (z - h(g\vk))^{-1}  dz \\
    & = P_{occ}(g\vk)
    \end{split}
\end{equation}
Hence $P_{occ}(\vk)^*$ and $P_{occ}(g\vk)$ have the same rank and $\{ D(g) \ket{u^*_{nk}} : n \in \mc{I}_{occ}\}$ is a complete orthogonal basis for the range of $P_{occ}(g\vk)$ as we wanted to show.

\section{Symmetries of the BM and interacting BM Model}
\label{sec:bm-symm}

\QZ{In this section, we introduce the matrix representation of the symmetry operation and discuss the discrete symmetries of the non-interacting BM model. These definitions help us get prepared for the following discussion about the projected IBM Hamiltonian in Section \ref{sec:ibm-symm} and the spontaneous symmetry breaking in Section \ref{sec:symm-broken}.}

%\QZ{In the single-valley, spinless system, we abbreviate the valley and spin dimension.} We introduce a multi-index $\alpha=(\vG,\sigma,l)$ to denote the ``internal variables'', i.e., the BM wavefunction is $u_{n\vk}(\alpha)$, and the total number of internal variables is $N_{\alpha}$. The action of a discrete symmetry operator $g$ on the fermion basis $\hat c^{\dag}_{\vk}(\alpha)$ is
%\begin{equation}
%g\hat{c}^{\dag}_{\vk}(\alpha)g^{-1} = \sum_{\alpha'} 
%\hat{c}^{\dag}_{g\vk}(\alpha') [D(g)]_{\alpha',\alpha}.
%\end{equation}
%The unitary matrix $D(g)\in \CC^{N_{\alpha}\times N_{\alpha}}$ is called the representation matrix.
%Similarly $g$ acting on the annihilation operators 
%\begin{equation}
%g\hat{c}_{\vk}(\alpha)g^{-1} = \sum_{\alpha'} 
%\hat{c}_{g\vk}(\alpha') [D(g)]^*_{\alpha',\alpha}.
%\end{equation}
%A symmetry $g$ is unitary if for any $c\in \CC$, $gcg^{-1}=c$. 
%A symmetry $g$ is antiunitary if for any $c\in \CC$, $gcg^{-1}=c^*$. 

For example, the $C_{3z}$ symmetry is unitary which maps the $\vK$ valley into an equivalent $\vK$ valley. Specifically, it maps $\vK+\vk\to \vK+C_{3z}\vk$.
So
\begin{equation}
(C_{3z})\hat{c}^{\dag}_{\vk}(\vG,\sigma,l)(C_{3z})^{-1} = \sum_{\alpha'}
\hat{c}^{\dag}_{C_{3z}\vk}(\vG',\sigma',l') [D(C_{3z})]_{\alpha',\alpha}.
\end{equation}
with
\begin{equation}
[D(C_{3z})]_{\vG'\sigma'l',\vG\sigma l} = \delta_{\vG',C_{3z}\vG} \delta_{l',l} \left(e^{\I \frac{2\pi}{3} \sigma_z}\right)_{\sigma',\sigma}.
\end{equation}
The $C_{2z}\mc{T}$ symmetry is antiunitary which maps $\vk\to \vk$
\begin{equation}
(C_{2z}\mc{T})\hat{c}^{\dag}_{\vk}(\vG,\sigma,l)(C_{2z}\mc{T})^{-1} = \sum_{\alpha'}
\hat{c}^{\dag}_{\vk}(\vG',\sigma',l') [D(C_{2z}\mc{T})]_{\alpha',\alpha}.
\end{equation}
with
\begin{equation}
[D(C_{2z}\mc{T})]_{\vG'\sigma'l',\vG\sigma l} = \delta_{\vG',\vG} \delta_{l',l} (\sigma_x)_{\sigma',\sigma}.
\end{equation}
 
The BM Hamiltonian commutes with both $C_{2z}\mc{T}$ and $C_{3z}$.

\section{Numerical verification of symmetries of the IBM model}
\label{sec:symm_ham}

According to the discussion in \cref{sec:ibm-symm}, the IBM model should inherit the symmetries of the BM Hamiltonian in the continuous limit. 
However, the discretized IBM model may not exactly satisfy such symmetry conditions, which may be due to the Brillouin zone discretization, truncation of the number of shells, and the treatment of the subtraction Hamiltonian etc. 
Therefore one should numerically verify whether the discretized IBM model satisfy the symmetry conditions. 
To this end, it is useful to have a gauge-invariant order parameter to quantify the symmetry breaking.

With the transformation rule set by the sewing matrices, we can check whether a quadratic Hamiltonian 
$\hat{A}=\sum_{\vk}\sum_{mn}[A(\vk)]_{mn} \hat{f}^{\dag}_{m\vk} \hat{f}_{n\vk}$
commutes with the symmetry $g$. 
If $g\hat{A}g^{-1}=\hat{A}$, and assume that the Monkhorst-Pack grid discretizing the mBZ is invariant under $g$, then
\begin{equation}
\begin{split}
g\hat{A}g^{-1}=&\sum_{\vk}\sum_{mn} [A(\vk)]_{mn}\sum_{pq} [B(g)]_{\vk,pm} [B(g)]^*_{\vk,qn} \hat{f}^{\dag}_{p,g\vk}\hat{f}_{q,g\vk}\\
=&\sum_{g\vk} \sum_{pq} \left([B(g)]_{\vk} A(\vk) [B(g)]_{\vk}^{\dag}\right)_{pq}\hat{f}^{\dag}_{p,g\vk}\hat{f}_{q,g\vk}.
\end{split}
\end{equation}

\LL{ Analogous to $\mc{C}_{\vk}(g)$, should we define a order parameter, e.g., $\mc{C}_{\vk}(g,A)$? That may be useful if we want to report the order parameter in the numerical section.} 
Therefore we have the relation 
\begin{equation}
[B(g)]_{\vk} A(\vk) [B(g)]^{\dag}_{\vk}-A(g\vk)=0.
\end{equation}
Similarly, if $g$ is antiunitary, then
\begin{equation}
[B(g)]^{\text{anti}}_{\vk} A^*(\vk) ([B(g)]^{\text{anti}}_{\vk})^{\dag}-A(-g\vk)=0.
\end{equation}

The same procedure can be used to check whether the quartic Hamiltonian commutes with $g$. \QZ{ As in \cref{eqn:subtracted_HF}, the single-particle term in the subtracted Hamiltonian is a quartic term. Therefore, the symmetries will be verified by setting $A(\vk)=h_s(\vk)$ in Section \ref{sec:ibm-symm}.}

\QZ{ For the coulomb interaction term,} due to the structure in \cref{eqn:interaction_simplify}, it is sufficient to verify that $g$ commutes with the pseudo-density operator $\hat{\rho}_{\vq}$ in \cref{eqn:rho_operator}, which is a quadratic operator.
Direct computation shows that if $g$ is unitary and commutes with $\hat{\rho}_{\vq}$,
then
\begin{equation}
[B(g)]_{\vk} \Lambda_{\vk}(\vq) [B(g)]^{\dag}_{\vk+\vq}-\Lambda_{g\vk}(g\vq)=0.
\end{equation}
If $g$ is antiunitary, then
\begin{equation}
[B(g)]^{\text{anti}}_{\vk} \Lambda^*_{\vk}(\vq) ([B(g)]^{\text{anti}}_{\vk+\vq})^{\dag}-\Lambda_{g\vk}(g\vq)=0.
\end{equation}

Using the strategy above, we can verify that $g\hat{H}_{\mathrm{IBM}}g^{-1}=\hat{H}_{\mathrm{IBM}}$ for $g=C_{2z}\mc{T},C_{3z}$ in the continuous limit. \QZ{ More details are in Section \ref{sec:ibm-symm}.} However, in a calculation with a finite number of $\vk$ points, the symmetry may be slightly broken. 
Therefore we need to check the norm of the commutators above to verify that the magnitude of the broken symmetry is sufficiently small. \QZ{ The definition of the norm and the discussion of symmetry breaking are discussed in Section \ref{sec:symm-broken}.}

% KDS: I think what you have below is good, but the operators $\hat{\vc}$ are already defined in Section III
%\QZ{ $\hat{\vc}_{n\vk}^\dag/\hat{\vc}_{n\vk}$ is the creation/annihilation operator defined in the space of combined indices $\alpha=(\vG, s,\sigma,\tau,l)$, including the Moir\'e reciprocal lattice vector, spin, sublattice, valley, layer, and $n$ represents the unique band index. Note that the combined indices $\alpha$ and band indices $n$ are correlated with each other.} Unlike unitary symmetries, the action of complex conjugation is defined with respect to a choice of basis. Recalling

\LL{ This belongs to \cref{sec:ibm-symm}?} 

In order to check the symmetries of the interacting BM model, we need to discuss the interacting term in \cref{eqn:interaction_simplify}. For unitary/antiunitary operator, it is sufficient to verify the symmetries of form factors:
$$
[\Lambda_{\vk}(\vq)]_{mn}=\braket{u_{m\vk}|u_{n,\vk+\vq}},
$$
where $u_{m\vk}$, $u_{n,\vk+\vq}$ are the flat bands in the BM band structure. It has been proven that the BM model has $C_{2z}\mc{T}$ symmetry. \LL{ This uses the Chern band basis, also seem obsolete?} Given a flat band $u_{m\vk}$, another band $D[g]u_{m\vk}$ is also a flat band. For example, two flat bands can be chosen as $u_{1,\vk}$ and $u_{-1,\vk}=\sigma_xu^*_{1,\vk}$. With this kind of setup, the flat bands always include the pairs of bands and each pair is connected by one specific symmetry. In this case, the symmetry operation using sewing matrix can also be ``closed'' and ``complete''. In Chern band basis $u_{\pm,\vk}=u_{\pm1,\vk}$, the sewing matrix is defined as $[B(C_{2z}\mathcal{T})]_{\vk,mn}=\braket{u_{m\vk}|\sigma_x|u^*_{n\vk}}=\braket{u_{m\vk}|u_{-n\vk}}=\delta_{m,-n}$. In random band basis $u_{\pm,\vk}=c_{\pm,1,\vk}u_{1,\vk}+c_{\pm,-1,\vk}u_{-1,\vk}$, the sewing matrix is $[B(C_{2z}\mathcal{T})]_{\vk,mn}=c^*_{m,-1,\vk}c^*_{n,1,\vk}+c^*_{m,1,\vk}c^*_{n,-1,\vk}$. It's easy to verify that these sewing matrices are ``closed'' and ``complete''.

Then for unitary operator, we have

\begin{equation}
\begin{split}
[[B(g)]^{\dag}_{\vk} \Lambda_{g\vk}(\vq) [B(g)]_{\vk+\vq}]_{mn}&=\sum_{m'n'}[B(g)]^{\dag}_{\vk,mn'} [\Lambda_{g\vk}(\vq)]_{n'm'}[B(g)]_{\vk+\vq,m'n},\\
&=\sum_{m'n'}[B(g)]^{\dag}_{\vk,mn'}\braket{u_{n',g\vk}|u_{m',g\vk+g\vq}}[B(g)]_{\vk+\vq,m'n}\\
&=\braket{u_{m\vk}|D^{\dag}(g)D(g)|u_{n,\vk+\vq}},\\
&=\braket{u_{m\vk}|u_{n,\vk+\vq}}=[\Lambda_{\vk}(\vq)]_{mn},
\end{split}
\end{equation}
and for antiunitary operator: 
\begin{equation}
\begin{split}
[([B(g)]^{\text{anti}}_{\vk})^{\dag} \Lambda_{g\vk}(\vq) [B(g)]^{\text{anti}}_{\vk+\vq}]_{mn}&=\sum_{m'n'}([B(g)]^{\text{anti}}_{\vk,mn'})^{\dag} [\Lambda_{g\vk}(\vq)]_{n'm'}[B(g)]^{\text{anti}}_{\vk+\vq,m'n},\\
&=\sum_{m'n'}([B(g)]^{\text{anti}}_{\vk,mn'})^{\dag}\braket{u_{n',g\vk}|u_{m',g\vk+g\vq}}[B(g)]^{\text{anti}}_{\vk+\vq,m'n}\\
&=\braket{u^*_{m\vk}|D^{\dag}(g)D(g)|u^*_{n,\vk+\vq}},\\
&=\braket{u^*_{m\vk}|u^*_{n,\vk+\vq}}=[\Lambda^*_{\vk}(\vq)]_{mn}.
\end{split}
\end{equation}

This holds for both BM and Chern band basis. To summarize, the flat bands connected by the desired symmetry should be included to form a complete set of basis in the projected space.

For the subtraction term in \cref{eqn:subtracted_HF}, it can be verified using
\begin{equation}
[B(g)]^{\dag}_{\vk}h_s(g\vk)[B(g)]_{\vk}=h_s(\vk),
\end{equation}
which is equivalent to verify that $[B(g)]^{\dag}_{\vk}\delta P^0(g\vk+g\vq)[B(g)]_{\vk}=\delta P^0(\vk+\vq)$ for unitary operator. Therefore, the symmetries of the subtracted Hamiltonian still holds if the reference density also have the same symmetries. Some common choice of the reference density includes: (i) the ground state density of the BM model; (ii) the ground state density of the decoupled BM model; (iii) the charge neural point ($\delta P^0=0$). All these choice share the same symmetries with BM model.
