# Supplementary material for: Interacting models for twisted bilayer graphene: a quantum chemistry approach
Source: arXiv:2211.09243 source file (2022-11-16)
Supplement: Supplementary file 2 [file appendix1.tex]

\begin{comment}
% According to prx paper, the form factor has the form:
% \begin{equation}
% \Lambda_{\vk}(G)=\begin{pmatrix}
% a&b\\
% b&a
% \end{pmatrix},
% \end{equation}
% with $a\gg b$ and $a,b$ depends on $G, \vk$.

The first term in \cref{eqn:subtraction} can be written as 
\begin{equation}
\sum_{\vG} V(\vG)\Lambda_{\vk}(G) \sum_{\vk'} \Tr[ \Lambda_{\vk'}(-\vG) \delta P^0(\vk')],
\end{equation}
where
\begin{equation}
\begin{split}
\Tr[ \Lambda_{\vk'}(-\vG) \delta P^0(\vk')]&=\sum_{mn}[\Lambda_{\vk'}(-\vG)]_{mn} [\delta P^0(\vk')]_{nm},\\
&=\sum_{mn}\braket{u_{m\vk'}|u_{n\vk'}}[\delta P^0(\vk')]_{nm},\\
&=\sum_{mn}\delta_{mn}[\delta P^0(\vk')]_{nm},\\
&=\Tr[\delta P^0(\vk')]=0.
\end{split}
\end{equation}

For half-filling system, we have $\Tr[\delta P^0(\vk')]=0$. 

\end{comment}
